# Supplementary material for: Phonon-enhanced strain sensitivity of quantum dots in two-dimensional semiconductors
Source: arXiv:2602.17212 ancillary file (2026-02-19)
Supplement: Supplementary file 1 [file suppl_iitgoasqup.pdf]

# Phonon-enhanced strain sensitivity of quantum dots in two-dimensional semiconductors

Sumitra Shit,[1] Yunus Waheed,[1] Jithin Thoppil Surendran,[1] Indrajeet Dhananjay Prasad,[1] Kenji Watanabe,[2] Takashi Taniguchi,[3] and Santosh Kumar[1]

[1)] *School of Physical Sciences, Indian Institute of Technology Goa, Ponda, 403401, Goa, India*

[2)] *Research Center for Electronic and Optical Materials, National Institute for Materials Science, 1-1 Namiki, Tsukuba 305-0044, Japan*

[3)] *Research Center for Materials Nanoarchitectonics, National Institute for Materials Science, 1-1 Namiki, Tsukuba, 305-0044, Japan*

(*Electronic mail: skumar@iitgoa.ac.in)

(Dated: 18 February 2026)

## SUPPORTING INFORMATION

## I. OBSERVATION OF STRAIN-INDUCED QUANTUM DOTS (QDS) IN 2D HETEROSTRUCTURES

### A. QDs in six heterostructure samples, containing ML-$WS_2$

Figure. S1 (a-c) shows $\mu$-PL peak intensity spatial maps for samples (a) S1, (b) C1, and (c) C2, where ML-$WS_2$ flakes are deposited on Si/$SiO_2$ substrates containing spherical nanoparticles (SNPs) for sample S1 and shape-engineered nanoparticles (ENPs) for samples C1 and C2. The regions under the dotted curves in each map represent light emission from ML-$WS_2$ regions of the flakes. Five points are highlighted within the ML region in the respective map, and their corresponding $\mu$-PL spectra are shown in the bottom panels. These ENP locations (in Fig. S1 (b) for C1 and Fig. S1 (c) for C2) are visible as red spots in the $\mu$-PL map and demonstrate significantly lower emission energies compared to those in sample S1. Similarly, Fig. S2 (a–c) presents the $\mu$-PL peak intensity spatial maps and spectra from selected locations in the bottom panels of samples (a) S2, (b) S3, and (c) S4. While samples S2 and S3 exhibit a typical emission distribution as reported previously[1], sample S4 shows a distinct red-shifted emission with larger local strain.

### B. QDs in three heterostructure samples, containing ML-$WSe_2$

Fig. S3 (a–c) presents the $\mu$-PL peak intensity spatial maps of samples (a) W1, (b) W2, and (c) S5, deposited on Si/$SiO_2$ either containing wrinkles or SNPs. The regions under the dotted curves in each map represent the light emission from the ML-$WSe_2$ regions of the flakes. Samples W1 and W2 contain unintentional wrinkles formed during the transfer process, resulting in naturally strained regions. In contrast, sample S5 contains SNPs beneath ML-$WSe_2$. Multiple strained locations were examined for each sample, and five representative points within the ML region are highlighted in each map; their corresponding $\mu$-PL spectra are shown in the bottom panels.

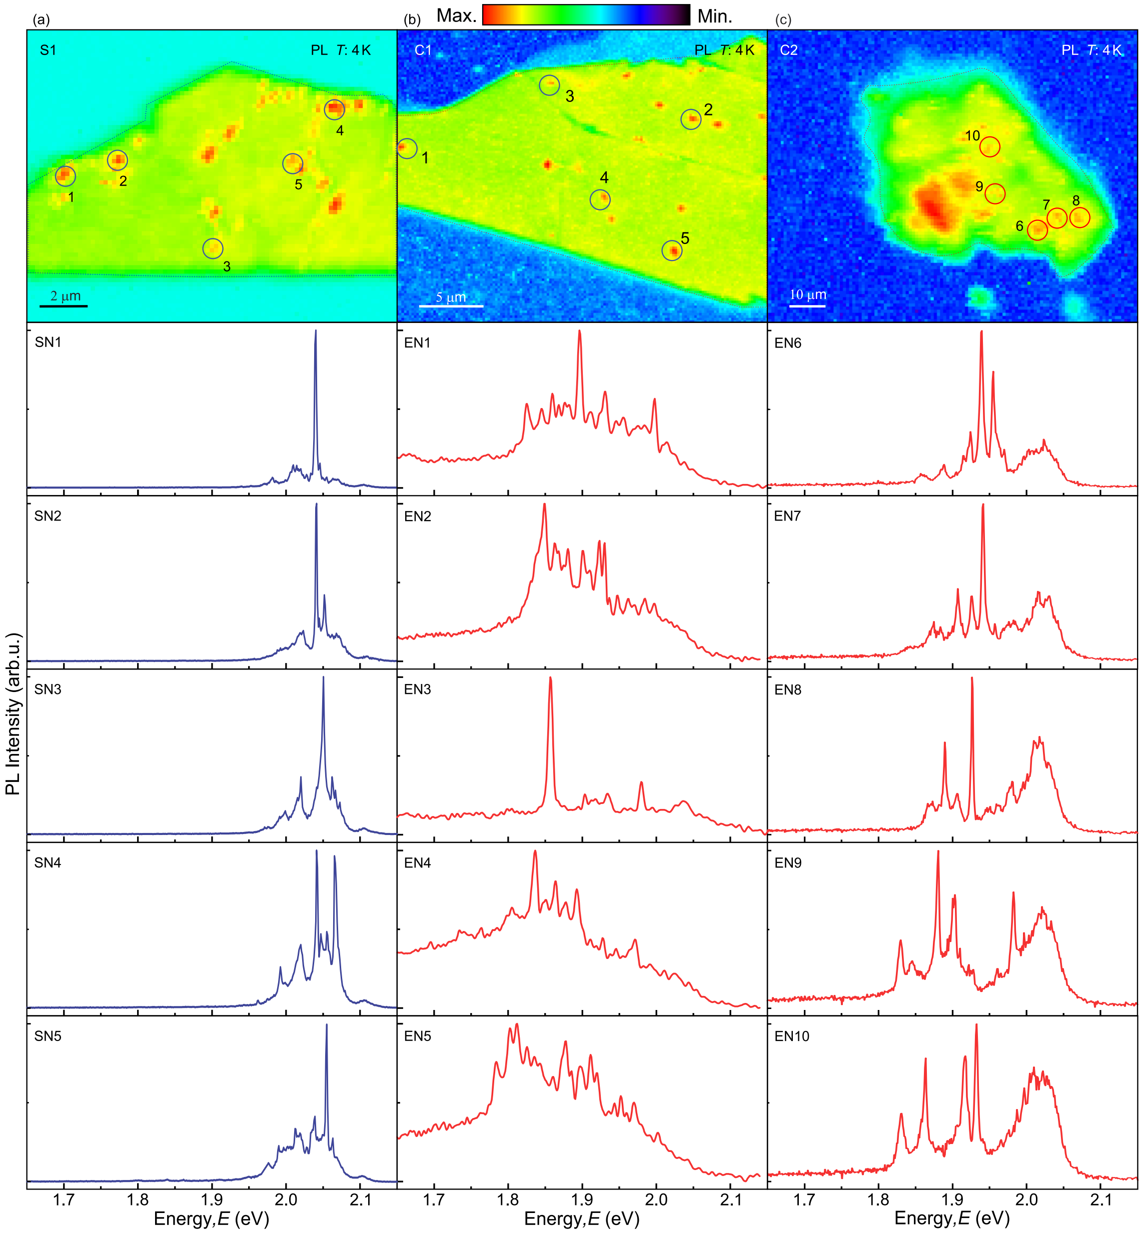


FIG. S1. **Strain-induced QDs emission energies in ML-$WS_2$ on SNPs and ENPs.** (a-c) The representative $\mu$-PL peak intensity spatial maps of samples (a) S1, (b) C1, and (c) C2, respectively; in the spectral window of 550-850 nm at low temperature (LT), T=4 K. Sample S1 contains ML-$WS_2$ on spherical NPs, whereas samples C1 and C2 use ENPs. Regions covered with dotted lines in (a-c) show light emission from ML-$WS_2$ regions of the flakes. The five spectra from the SNP and ENP locations are shown in the bottom panels for the respective samples.

## II. ROOM TEMPERATURE (RT) LOCAL-STRAIN AT THE NP LOCATION VIA μ-RAMAN AND $\mu$-PL SPECTROSCOPY:

Figure. S4 (a) compares the Raman spectra of ML-$WS_2$ taken at the EN2 location (open diamonds) and the flat region (closed diamonds) in sample C1. These spectra were fitted (solid lines) with a multi-Lorentzian function for extracting the Raman shifts of six identified phonon modes. The vertical dotted (solid) lines mark Raman shifts for the EN2 (flat) location, respectively. These measured values, along with literature values for unstrained ML-$WS_2$[2], are listed in Table S1.

The Raman shifts observed in the flat region match those of unstrained ML-$WS_2$, confirming that this region is strain-free. In contrast, significant changes in Raman shifts of these six phonon modes are observed at the EN2 location, indicating the presence of local strain. We measure a biaxial local strain of $0.72 \pm 0.07\%$ at this location, using the known shift-rate of the 2LA(M) phonon mode of ML-$WS_2$ (-6.3 $cm^{-1}$/% biaxial strain). The 2LA(M) mode is chosen because it is minimally affected by charge-carrier doping[3,4].

The PL spectrum of ML-$WS_2$ from the same EN2 location, shown in Fig. S4 (b), further support this observation. A thick blue curve fitted using a Gaussian function represents the delocalized neutral exciton (2D-$X^0$), while a thin red curve fitted with a Lorentzian represents the negative trion (2D-$X^-$) emission. The dotted vertical line marks the 2D-$X^0$ emission energy of ML-$WS_2$ at the EN2 location, that is redshifted by $\sim$35 meV from the 2D-$X^0$ emission energy of unstrained[4] ML-$WS_2$ (also marked by a solid vertical line). Utilizing the 2D-$X^0$ gauge factor of $-38 \pm 3.0$ meV/% biaxial local-strain [4], we obtained a local strain of $0.93 \pm 0.07\%$ in ML-$WS_2$ at the EN2 location in Sample C1. We measured both Raman and PL spectra from multiple such locations in Sample C1. A PL spatial map of the complete flake, shown in Fig. S5 (d), highlights all these locations. The extracted local-strain values using both Raman and PL methods are shown in Fig. S4 (c) where method-dependent small variations in the strain values of each location can be seen. Figure S4 (d) shows a histogram of these variations with a standard deviation of 0.15%, underscoring the reliability of both strain quantification methods. Thus, we utilized strain estimated using PL method for understanding the properties of QDs in ML-$WS_2$ and ML-$WSe_2$ from various samples. Fig. S6 presents histogram of strains measured at various locations in sample S1.

The errors in Fig. S4 (c) for PL and Raman are estimated using equations 1 and 2, respectively.

$$\Delta\varepsilon_{PL} = \varepsilon_{PL} \times \sqrt{\left(\frac{\Delta E_{err}}{\Delta E}\right)^2 + \left(\frac{G_{err}}{G}\right)^2}, \qquad (1)$$

$$\Delta\varepsilon_R = \varepsilon_R \times \sqrt{\left(\frac{\Delta\nu}{\nu}\right)^2 + \left(\frac{r_{\text{err}}}{r}\right)^2}, \tag{2}$$

where $\Delta\varepsilon$ is the error in strain and $\varepsilon$ is the corresponding calculated strain. $\Delta E$ is the strain-induced shift in the 2D-$X^0$ emission energy, and $\Delta E_{\text{err}}$ is its associated error. G and $G_{\text{err}}$ show the gauge factor and its error, respectively. $\nu$ is a Raman peak shift due to strain, $\Delta\nu$ is the corresponding error. For both $\Delta E_{\text{err}}$ and $\Delta\nu$, the larger of the experimental error and the fitting error is used as the error bar. $r$ is the shift rate of the Raman mode and $r_{\text{err}}$ is the error in shift rate of the Raman mode taken from literature.

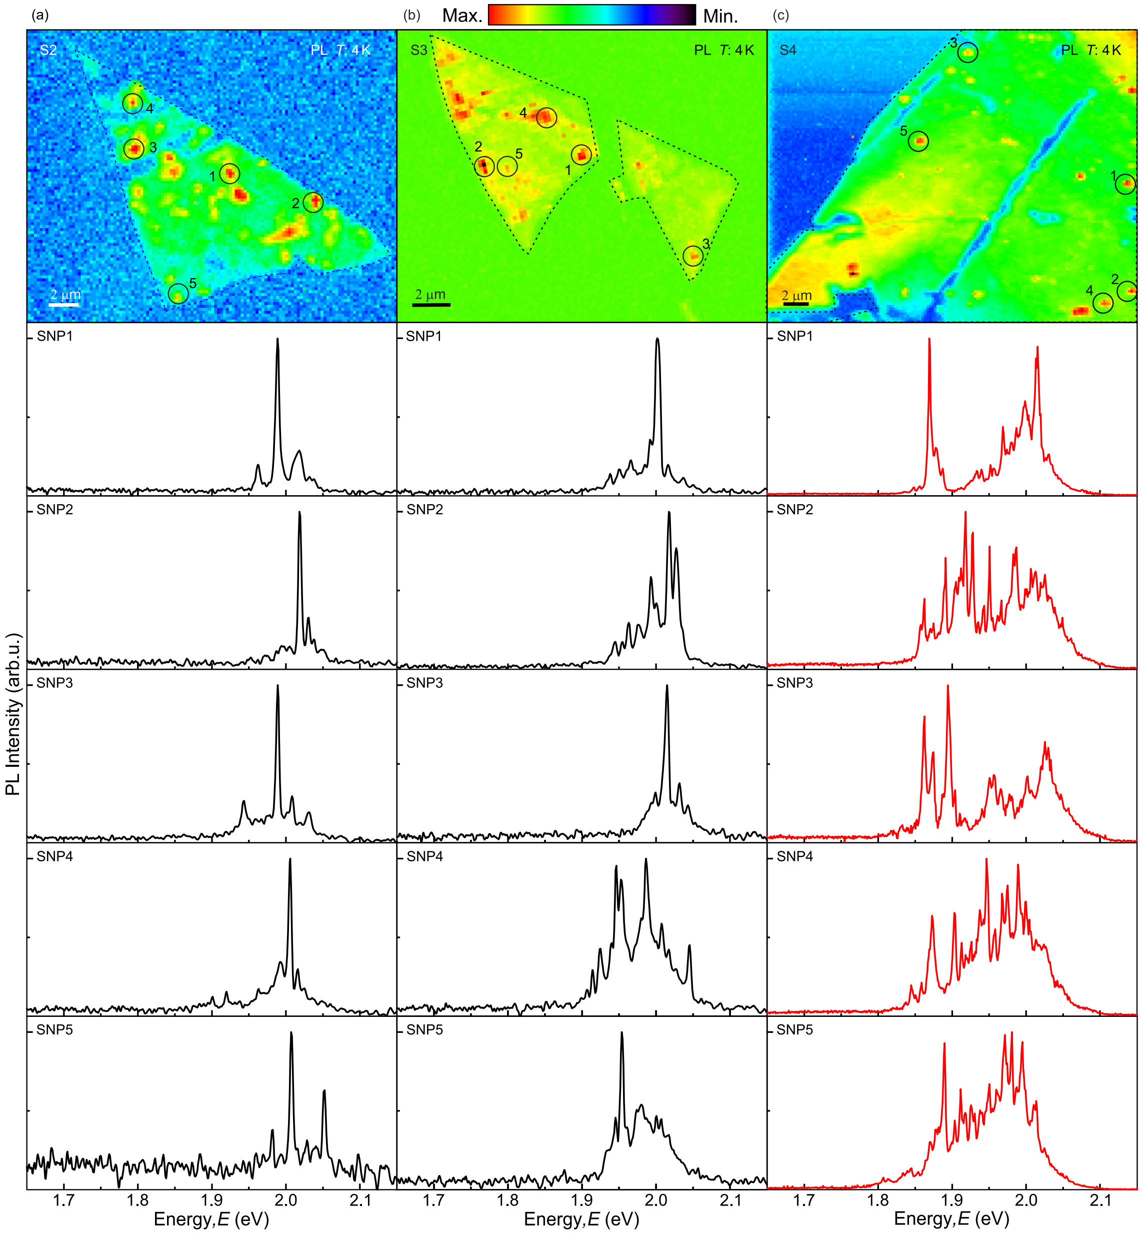


FIG. S2. **Strain-induced QDs emission energies in ML-$WS_2$ on SNPs.** (a-c) The representative $\mu$-PL peak intensity spatial maps of samples (a) S2, (b) S3, and (c) S4, respectively; in the spectral window of 550-850 nm at LT. Regions covered with dotted lines in (a-c) show light emission from ML-$WS_2$ regions of the flakes. The five spectra from the SNP locations are shown in the bottom panels for the respective samples.

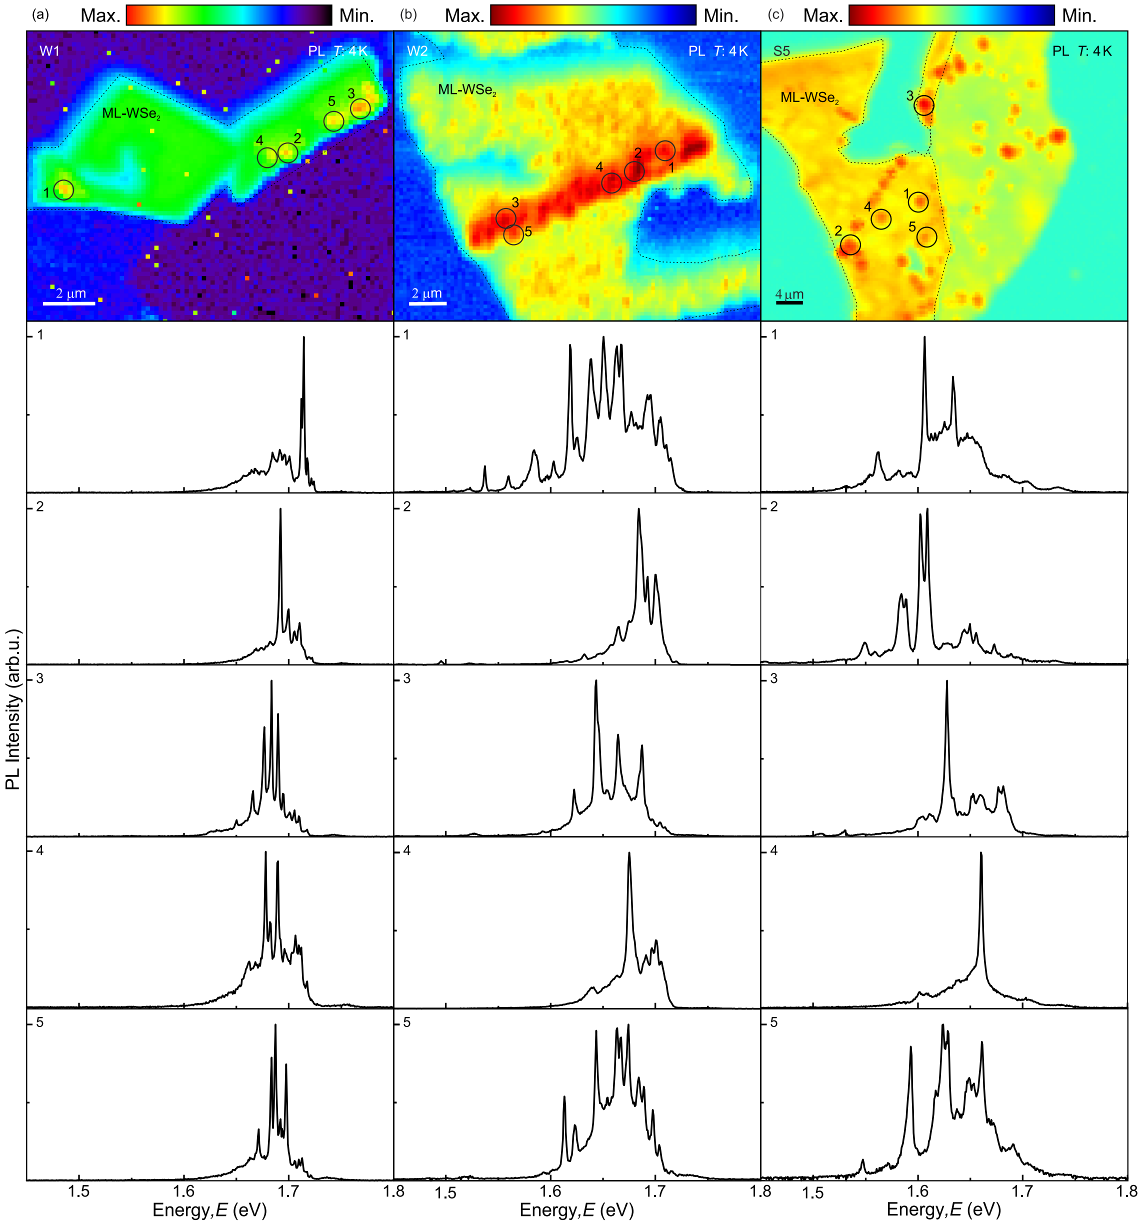


FIG. S3. **Strain-induced QDs emission energy in ML-WSe$_2$ due to wrinkles and SNPs.** The $\mu$-PL peak intensity spatial maps of ML-WSe$_2$ at LT, with the regions covered with dotted line, show unintentional wrinkles creating strained location of samples (a) W1, (b) W2, and strain created by SNPs in sample (c) S5 respectively; in the spectral window of 700-750 nm for sample W1, 700-770 nm for sample W2, and 700-800 nm for sample S5. The five spectra from the strained locations are shown in the bottom panels for each sample.

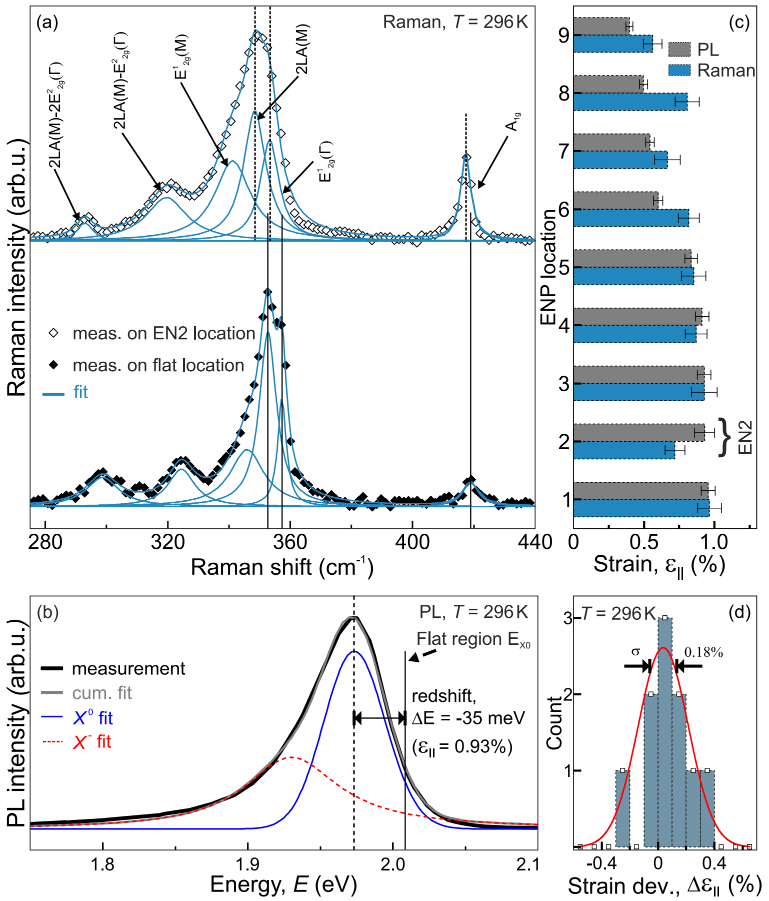


FIG. S4. **RT local-strain at the NP location via μ-Raman and $\mu$-PL spectroscopy:** (a) μ-Raman spectra of ML-$WS_2$ taken at EN2 (open diamonds, top) and flat-region (closed diamonds, bottom)locations in sample C1. Six Raman modes are labeled, and their frequencies are marked by vertical dotted (solid) lines corresponding to the EN2 (flat-region) location. (b) $\mu$-PL spectrum of ML-$WS_2$ taken at the CN location in sample C1. Solid thick lines are the fits. The neutral exciton, $\left(X^0\right)$ (negative trion, $\left(X^-\right)$) emission is shown as a thin dotted (thin solid) curve. (c) Bar plot comparing measured local strains values measured at 10 different ENP locations on ML-$WS_2$ in Sample C1 using Raman (thin bars) and PL (thick bars) spectroscopy. (d) Histogram showing the deviations in strain values obtained from the two measurement techniques (Raman and PL spectroscopy) of strain estimations (bin size: 0.10%). Error bars in (c) are described in the section C.

| | | Raman shift of mode $(\mathrm{cm}^{-1})$ | | | | | |
|---|---|---|---|---|---|---|---|
| | | $\mathbf{A_{1g}}$ | $\mathbf{E^1_{2g}(\Gamma)}$ | **2LA(M)** | $\mathbf{E^1_{2g}(M)}$ | $\mathbf{2LA(M) - E^2_{2g}(\Gamma)}$ | $\mathbf{2LA(M) - 2E^2_{2g}(\Gamma)}$ |
| **ML-$WS_2$** | **Raman shift: Literature**[2] | 419.00 | 357.00 | 353.00 | 347.00 | 325.00 | 298.00 |
| | **Flat region in sample C1** | 418.95 | 357.35 | 352.75 | 345.90 | 325.45 | 298.70 |
| | **EN2 location in sample C1** | 417.40 | 353.35 | 348.45 | 341.25 | 319.60 | 292.80 |

TABLE S1. Raman shifts values of six Raman modes taken from the literature[2] and measured at highly strained EN2 location and flat region in ML-$WS_2$ in Sample C1

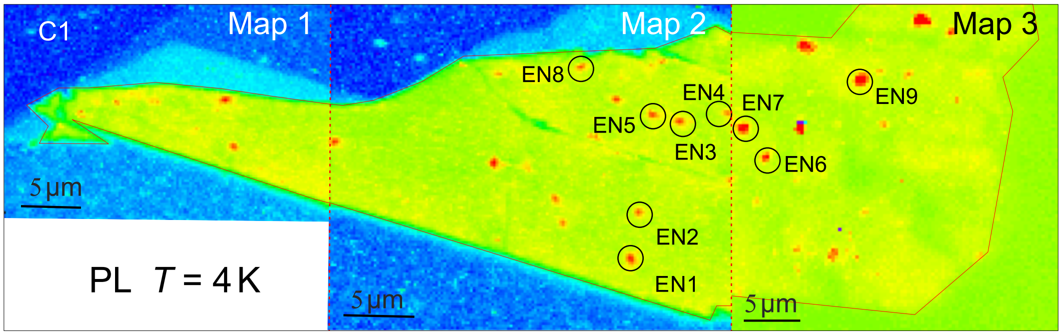


FIG. S5. **$\mu$-PL peak intensity spatial map of ML-$WS_2$ in sample C1.** The $\mu$-PL peak intensity spatial map of ML-$WS_2$ at LT with ENPs underneath. Three separate PL maps are combined to map the complete flake. The combined map also highlighting 9 different locations where Raman spectroscopy measurements were performed for calibrating the strain measured through PL measurements.

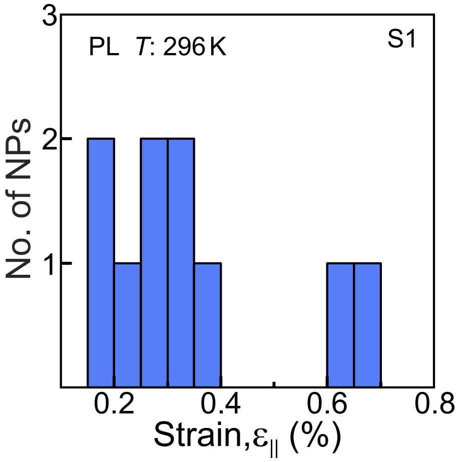


FIG. S6. **Range of strain across the ML-$WS_2$ region of sample S1 from PL analysis.** A histogram of measured strain values from multiple strained locations across the ML-$WS_2$ region of sample S1 estimated using PL spectroscopy (bin size = 0.05 %), shows the strain range throughout the sample.

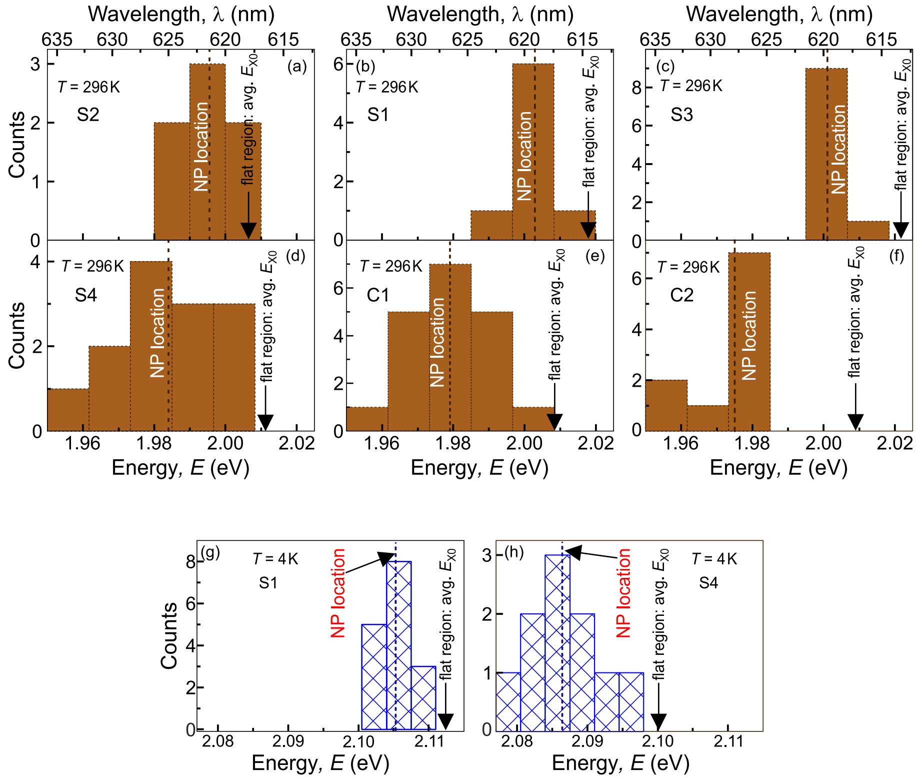


FIG. S7. **Statistical estimation of strain from 2D-$X^0$ emission energies in ML-$WS_2$ using $\mu$-PL spectroscopy at RT and 4K.** (a-f) Histograms of 2D-$X^0$ emission energies from multiple strained locations of 6 different samples at RT, showing the average peak energy of strained location (horizontal dotted line) and average flat region by arrow (bin size: 11 meV). (g-h) Histograms of 2D-$X^0$ emission energies from multiple strained locations of samples S1 and S4 at 4 K (bin size: 3.5 meV).

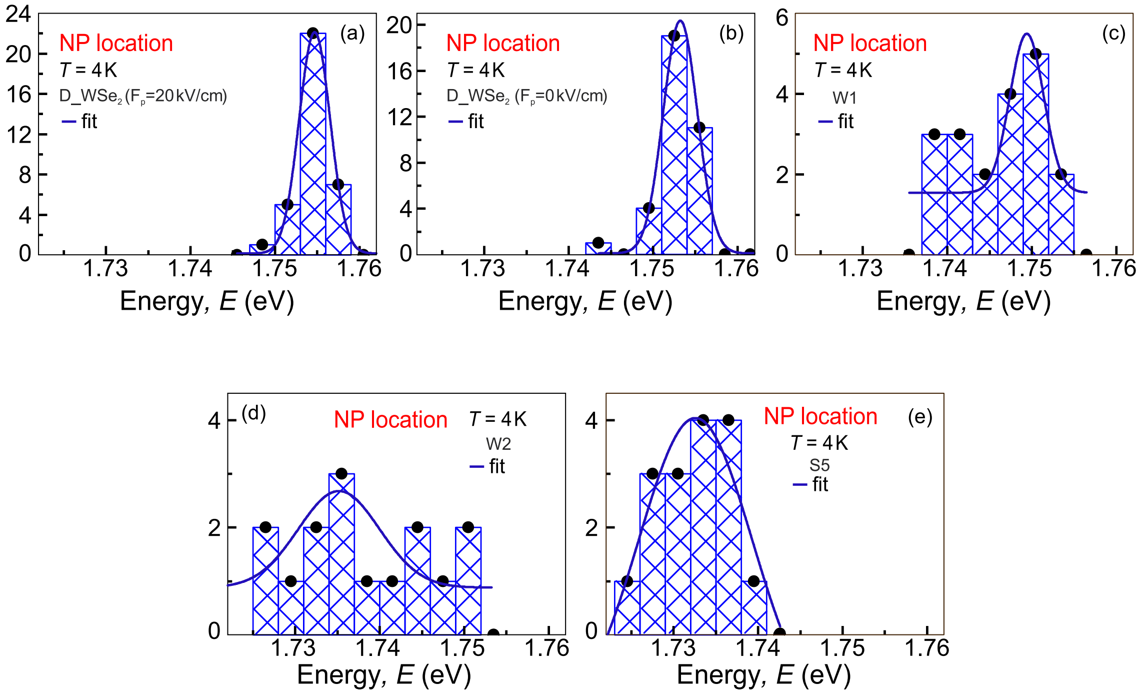


FIG. S8. **Statistical estimation of strain from 2D-$X^0$ emission energies in ML-$WSe_2$ using $\mu$-PL spectroscopy at 4 K.** (a-e) Histograms of 2D-$X^0$ emission energies from multiple strained locations of 4 different samples at 4 K (bin size:3 meV). The solid lines are Gaussian function fits.

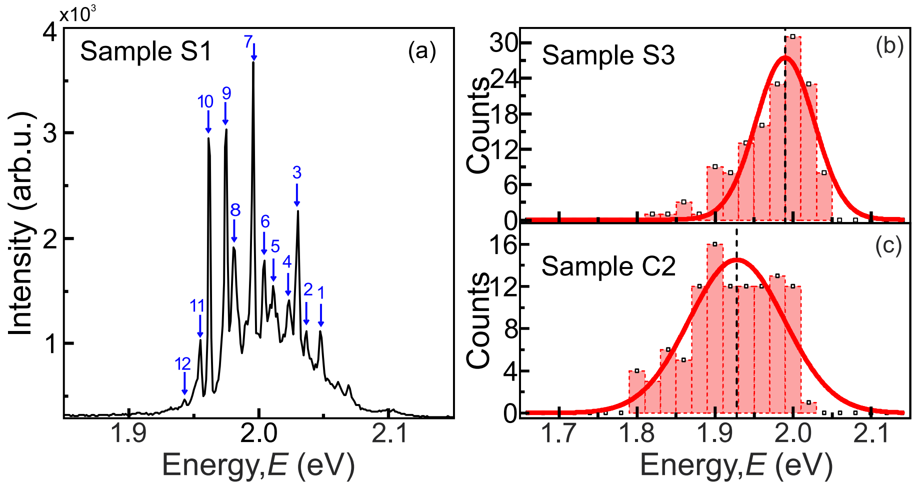


FIG. S9. **Statistical analysis of QD emission energies in ML-$WS_2$ samples.** (a) Representative $\mu$-PL spectrum acquired at a single NP location in ML-$WS_2$ from sample S1, showing multiple QD emission lines marked by numbers. (b-c) Histograms of QD emission energies measured at distinct strained locations in samples (b) S3 and (c) C2 (bin size:20 meV). The solid lines are Gaussian function fits.

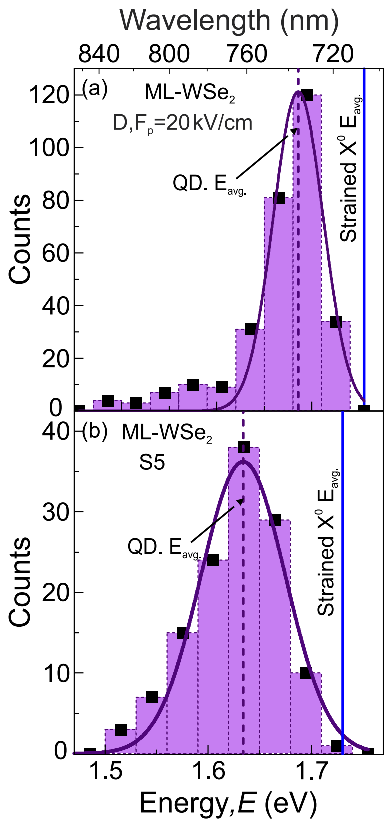


FIG. S10. **Statistical analysis of QD emission energies in ML-WSe$_2$.** (a-b) Histograms of QD emission energies from (a) piezo-device D, at $F_p = 20\,\mathrm{kV\,cm^{-1}}$ and (b) sample S5 (bin size = 30 meV).

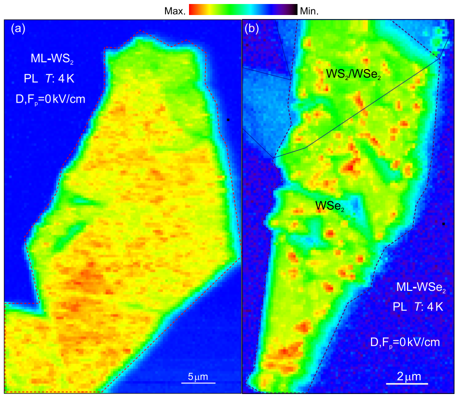


FIG. S11. **Strain-induced $\mu$-PL spatial maps in piezo-device D at 4 K.** (a-b) Representative $\mu$-PL peak intensity spatial map of (a) ML-WS$_2$ and (b) ML-WSe$_2$ in piezo-device D, in the spectral window of 590-700 nm for ML-WS$_2$ and 700-850 nm for ML-WSe$_2$ at $F_p = 0\,\mathrm{kV\,cm^{-1}}$, respectively.

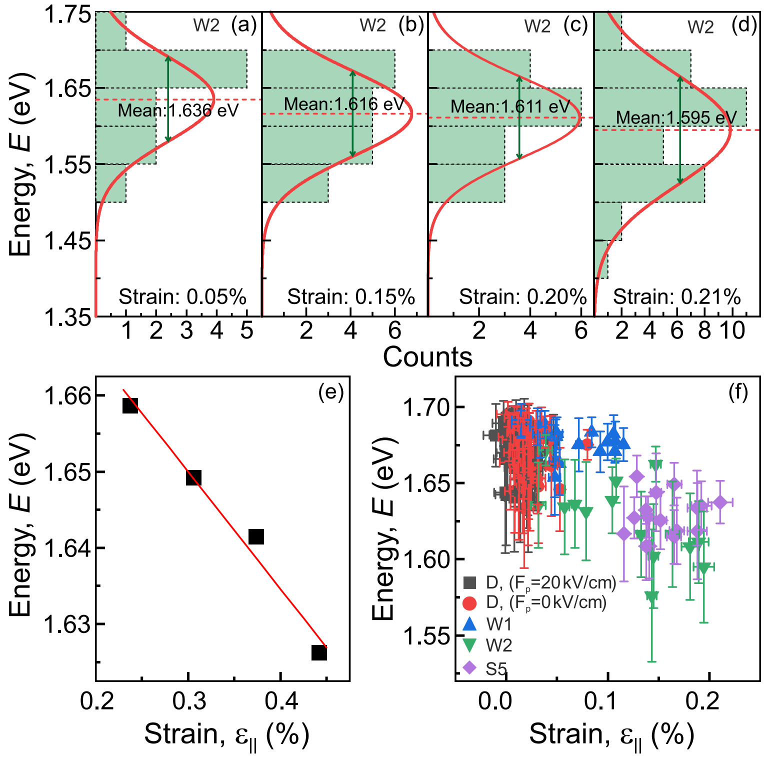


FIG. S12. **Correlation of ML-$WSe_2$ QD ensembles tuning with local strain at 4 K.** (a-d) Histograms of QD emission energies from 4 different strained locations, showing peak energy (horizontal dotted line) shift to lower energy as tensile strain increases (bin size: 50 meV). Solid curves are the Gaussian distribution fit. (e) Plot of 2D-$X^0$ emission energies of ML-$WSe_2$ as a function of strain, determining the strain energy-gauge factor of -153.8 ± 16.8 meV/%. Here, the emission energies and corresponding strain values were extracted from the work of Roy et al.[5]. (f) The average QD-ensemble emission energy at individual strained location was plotted as a function of local strain for various $WSe_2$ samples, revealing a systematic shift in emission energy with increasing strain.

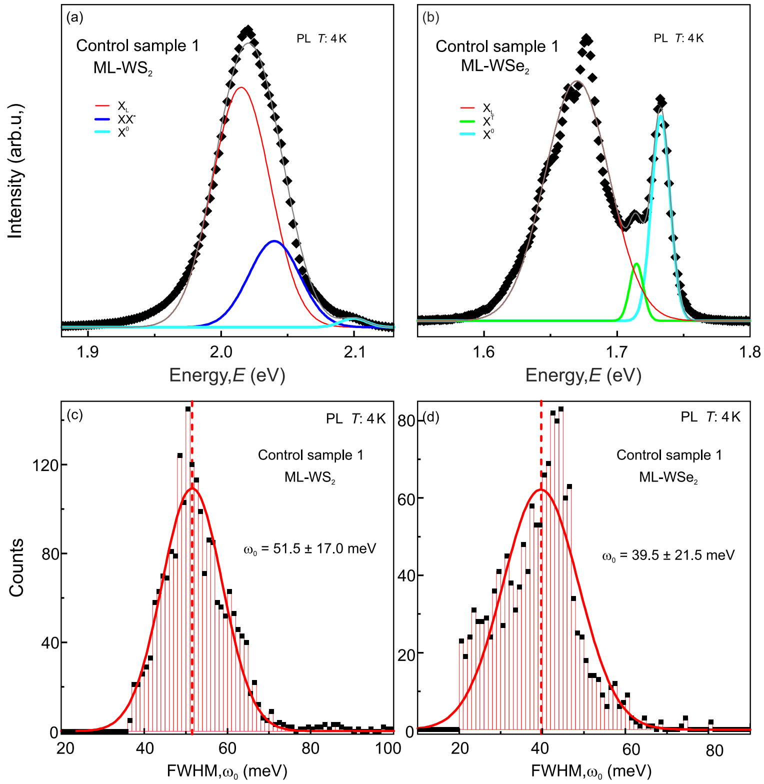


FIG. S13. **Ensemble width of localized exciton at 4 K on unstrained region.** A combined spectrum from a small unstrained-area $\mu$-PL map of (a) ML-$WS_2$ and (b) ML-$WSe_2$, fitted with 3 Gaussian peaks. Histograms of linewidth (FWHMs) of $X_L$ from(c) ML-$WS_2$ and (d) ML-$WSe_2$ showing small in-homogeneous broadening of $X_L$ emission lines from various unstrained location. The bin sizes: 1 meV.

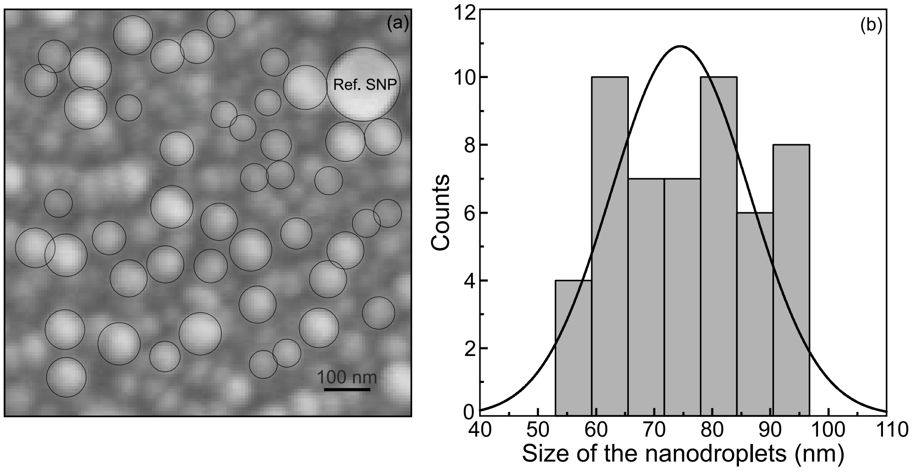


FIG. S14. **Statistics of sizes of NDs.** (a) SEM image of e-beam deposited (rate: $3.2 \pm 1.5$ Å/s) $SiO_x$ on Au-coated PMN-PT substrate, showing the formation of NDs, and (b) histogram of the ND diameter distribution, measured using the reference SNP (Ref. SNP) diameter, along with the corresponding normal distribution fit.

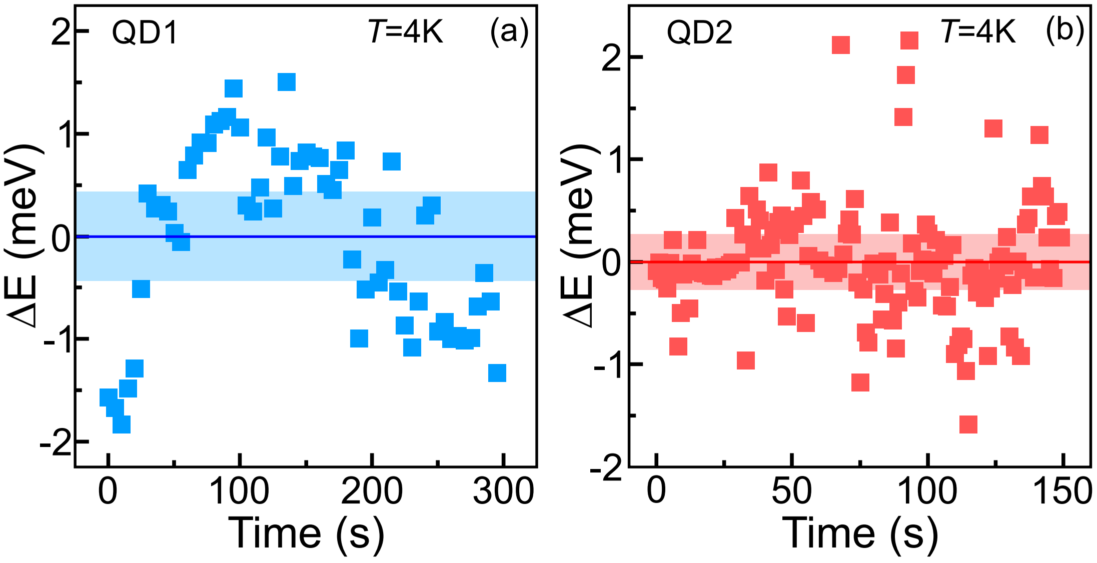


FIG. S15. **Energy jittering of QDs in ML-$WS_2$.** Time-dependent changes in emission energy relative to mean emission energy of (a) QD1 and (b) QD2 in ML-$WS_2$ from piezo-device D. The shaded region in both panels represents the one-sigma deviation, which is taken as the error bar associated with the mean emission energy.

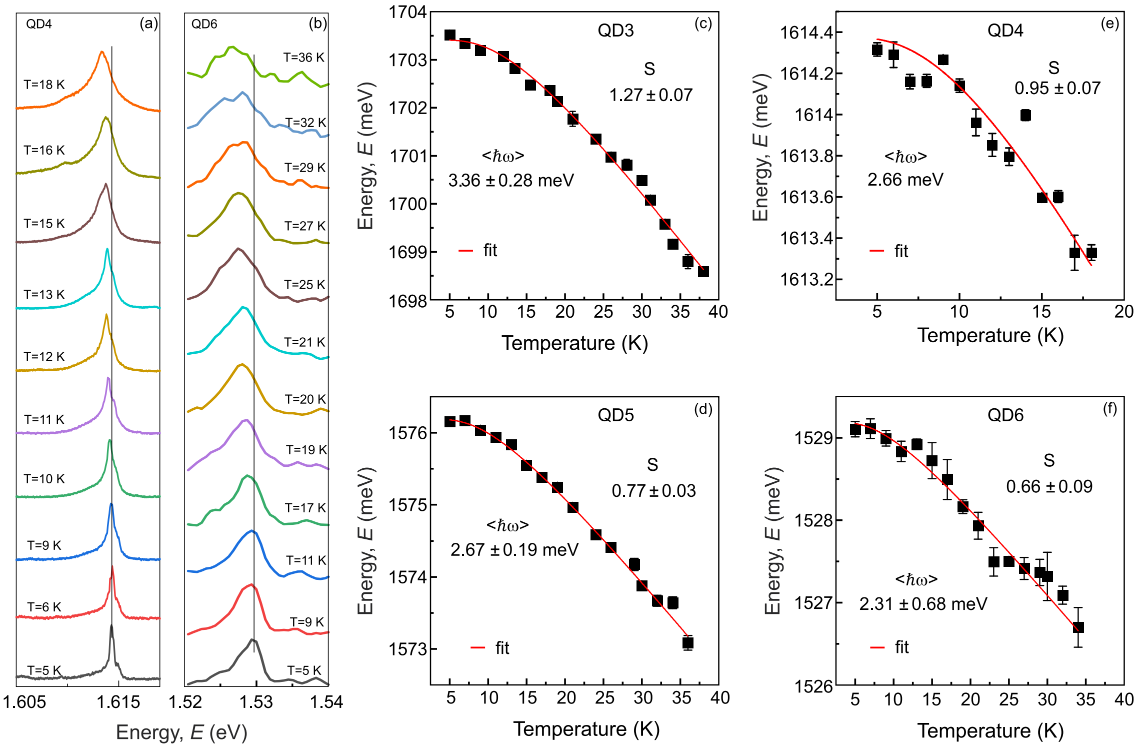

FIG. S16. **Temperature-dependent variation of emission energy of QDs in ML-WSe$_2$.** (a-b) Representative temperature dependent $\mu$-PL spectra in ML-WSe$_2$ for (a) QD4 and (b) QD6, illustrating the gradual shift in peak position from higher to lower energy. (c-f) Temperature dependent emission energy of (c) QD3, (d) QD5, (e) QD4, and (f) QD6 in ML-WSe$_2$, representing different shift rates and fitted by O'Donnell–Chen equation.

| Name of QDs/2D-$X^0$ | Physical parameter extracted from equation (1) | | |
|---|---|---|---|
| | $E_0$ (eV) | $\langle \hbar\omega \rangle$ (meV) | S |
| 2D-$X^0$ | 1.744 | $13.35 \pm 0.36$ | $2.29 \pm 0.08$ |
| QD3 | 1.703 | $3.36 \pm 0.28$ | $1.27 \pm 0.07$ |
| QD4 | 1.614 | 2.66 | $0.95 \pm 0.07$ |
| QD5 | 1.576 | $2.67 \pm 0.19$ | $0.77 \pm 0.03$ |
| QD6 | 1.529 | $2.31 \pm 0.68$ | $0.66 \pm 0.09$ |

TABLE S2. Temperature-dependent fitting parameters of 2D-$X^0$ and four QDs using the O'Donnell–Chen equation.

| Name of QDs | Method used | QD gauge factor (meV/% biaxial strain) |
|---|---|---|
| GaAs/AlGaAs | Biaxial | 70.0[6] |
| InGaAs/GaAs | Biaxial | 50.0[7] |
| | uniaxial | 67[8] |
| $In_xGa_{1-x}N/GaN$ | Theory | 110.0-64.4 (x=0.25-1)[9] |
| $WSe_2$ | Biaxial | 33.3 (100 PMN-PT)[10] |
| | Biaxial | 26 (001 PMN-PT)[11] |
| | Biaxial | 120 (110 PMN-PT)[10] |
| $WS_2$ (this work) | Biaxial | 76 (100 PMN-PT) |
| | Biaxial | 149±57 |
| $WSe_2$ (This work) | Biaxial | 275±123 |

TABLE S3. Summary of biaxial Gauge factor from various QD platform.

## REFERENCES


[1] J. T. Surendran, Y. Waheed, S. Shit, I. D. Prasad, K. Watanabe, T. Taniguchi, and S. Kumar, "Nanoparticle stressor-induced single-photon sources in monolayer $WS_2$ emitting into a narrowband visible spectral range," 2D Mater. **11**, 031002 (2024).

[2] X. Zhang, X.-F. Qiao, W. Shi, J.-B. Wu, D.-S. Jiang, and P.-H. Tan, "Phonon and raman scattering of two-dimensional transition metal dichalcogenides from monolayer, multilayer to bulk material," Chem. Soc. Rev. **44**, 2757–2785 (2015).

[3] A. Michail, D. Anestopoulos, N. Delikoukos, S. Grammatikopoulos, S. A. Tsirkas, N. N. Lathiotakis, O. Frank, K. Filintoglou, J. Parthenios, and K. Papagelis, "Tuning the photoluminescence and Raman response of single-layer $WS_2$ crystals using biaxial strain," J. Phys. Chem. C. **127**, 3506–3515 (2023).

[4] Y. Waheed, S. Shit, J. T. Surendran, I. D. Prasad, K. Watanabe, T. Taniguchi, and S. Kumar, "Large trion binding energy in monolayer $WS_2$ via strain-enhanced electron–phonon coupling," Commun. Mater. **6**, 86 (2025).

[5] S. Roy, J. Gao, and X. Yang, "Upconversion photoluminescence of monolayer $WSe_2$ with biaxial strain tuning," Opt. Express **32**, 3308–3315 (2024).

[6] S. Kumar, R. Trotta, E. Zallo, J. Plumhof, P. Atkinson, A. Rastelli, and O. G. Schmidt, "Strain-induced tuning of the emission wavelength of high quality GaAs/AlGaAs quantum dots in the spectral range of the 87Rb D2 lines," Appl. Phys. Lett. **99** (2011).

[7] R. Trotta, P. Atkinson, J. Plumhof, E. Zallo, R. O. Rezaev, S. Kumar, S. Baunack, J. Schröter, A. Rastelli, and O. G. Schmidt, "Nanomembrane quantum-light-emitting diodes integrated onto piezoelectric actuators." Advanced materials (Deerfield Beach, Fla.) **24**, 2668–2672 (2012).

[8] S. Seidl, M. Kroner, A. Högele, K. Karrai, R. J. Warburton, A. Badolato, and P. M. Petroff, "Effect of uniaxial stress on excitons in a self-assembled quantum dot," Appl. Phys. Lett. **88** (2006).

[9] A. S. Jbara, Z. Othaman, and M. Saeed, "Effect of size and indium-composition on linear and nonlinear optical absorption of InGaN/GaN lens-shaped quantum dot," Chin. Phys. B **25**, 057801 (2016).

[10] O. Iff, D. Tedeschi, J. Martín-Sánchez, M. Moczała-Dusanowska, S. Tongay, K. Yumigeta, J. Taboada-Gutiérrez, M. Savaresi, A. Rastelli, P. Alonso-González, *et al.*, "Strain-tunable single photon sources in $WSe_2$ monolayers," Nano Lett. **19**, 6931–6936 (2019).

[11] C. Chakraborty, A. Mukherjee, H. Moon, K. Konthasinghe, L. Qiu, W. Hou, T. Peña, C. Watson, S. M. Wu, D. Englund, *et al.*, "Strain tuning of the emission axis of quantum emitters in an atomically thin semiconductor," Optica **7**, 580–585 (2020).
